# Supplementary material for: Polarisation Control of Nanoantenna Cold Spots
Source: arXiv:2103.02544 source file (2021-03-03)
Supplement: Supplementary file 1 [file supplemental_material_arxiv.pdf]

# Supplemental Material: Formulation of the Linear System of Equations

Two plane waves, with electric field vectors expressed fully by two appropriate basis vectors, have two component amplitudes each: $x_1$ and $x_2$, and $x_3$ and $x_4$ respectively. The total electric field at a point $\mathbf{r}_0$ somewhere around a scatterer (or combination of scatterers), where we wish to create a cold spot, can be written as,

$$\mathbf{E}_{\mathrm{t}}(\mathbf{r}_0) = x_1\mathbf{E}_1(\mathbf{r}_0) + x_2\mathbf{E}_2(\mathbf{r}_0) + x_3\mathbf{E}_3(\mathbf{r}_0) + x_4\mathbf{E}_4(\mathbf{r}_0) \qquad (1)$$

The vector $\mathbf{E}_i(\mathbf{r}_0)$ is the electric field developed in the presence of and scaled by the plane wave component $x_i$. When a cold spot is created at $\mathbf{r}_0$, $\mathbf{E}_{\mathrm{t}}(\mathbf{r}_0) = 0$ and in its matrix form,

$$\overleftrightarrow{\mathbf{A}}\mathbf{x} = 0 \qquad (2)$$

Where $\overleftrightarrow{\mathbf{A}}$ is the $3 \times 4$ matrix whose $i^{\mathrm{th}}$ column is the electric field $\mathbf{E}_i(\mathbf{r}_0)$, and $\mathbf{x}$ contains $x_i$,

$$\overleftrightarrow{\mathbf{A}} = \begin{pmatrix} \uparrow & \uparrow & \uparrow & \uparrow \\ \mathbf{E}_1(\mathbf{r}_0) & \mathbf{E}_2(\mathbf{r}_0) & \mathbf{E}_3(\mathbf{r}_0) & \mathbf{E}_4(\mathbf{r}_0) \\ \downarrow & \downarrow & \downarrow & \downarrow \end{pmatrix} \qquad (3a)$$

$$\mathbf{x} = \begin{pmatrix} x_1 \\ x_2 \\ x_3 \\ x_4 \end{pmatrix} \qquad (3b)$$

The solution (3b) of (2) is the null space of $\overleftrightarrow{\mathbf{A}}$. Our goal, then, is to find the electric fields $\mathbf{E}_i(\mathbf{r}_0)$ so that (2) may be solved for any cold spot position vector $\mathbf{r}_0$.

## Incident Fields

The incoming plane waves can be expressed with two components, each in the direction of a suitable basis vector $\hat{\mathbf{e}}_i$,

$$\mathbf{E}_{\mathrm{a}}(\mathbf{r}) = (x_1\hat{\mathbf{e}}_1 + x_2\hat{\mathbf{e}}_2)\mathrm{e}^{\mathrm{i}\mathbf{k}_{\mathrm{a}}\cdot\mathbf{r}} \qquad (4a)$$

$$\mathbf{E}_{\mathrm{b}}(\mathbf{r}) = (x_3\hat{\mathbf{e}}_3 + x_4\hat{\mathbf{e}}_4)\mathrm{e}^{\mathrm{i}\mathbf{k}_{\mathrm{b}}\cdot\mathbf{r}} \qquad (4b)$$

Where $\hat{\mathbf{e}}_i$ is a $3 \times 1$ column vector detailing how much a plane wave component points along the cartesian basis vectors, and, travelling in free space, the plane waves' propagation vectors $\mathbf{k}_{\mathrm{a}}$ and $\mathbf{k}_{\mathrm{b}}$ are,

$$\mathbf{k}_\mathrm{a} = k_{\mathrm{a}x}\hat{\mathbf{x}} + k_{\mathrm{a}y}\hat{\mathbf{y}} + k_{\mathrm{a}z}\hat{\mathbf{z}} \qquad (5a)$$

$$\mathbf{k}_\mathrm{b} = k_{\mathrm{b}x}\hat{\mathbf{x}} + k_{\mathrm{b}y}\hat{\mathbf{y}} + k_{\mathrm{b}z}\hat{\mathbf{z}} \qquad (5b)$$

and,

$$\mathbf{k}_\mathrm{a} \cdot \mathbf{k}_\mathrm{a} = \mathbf{k}_\mathrm{b} \cdot \mathbf{k}_\mathrm{b} = k_0^2 = \left(\frac{2\pi}{\lambda_0}\right)^2 \qquad (5c)$$

Added together, plane waves $\mathbf{E}_\mathrm{a}(\mathbf{r})$ and $\mathbf{E}_\mathrm{b}(\mathbf{r})$ make up the incident field,

$$\mathbf{E}_\mathrm{inc}(\mathbf{r}) = x_1 \mathrm{e}^{\mathrm{i}\mathbf{k}_\mathrm{a}\cdot\mathbf{r}}\hat{\mathbf{e}}_1 + x_2 \mathrm{e}^{\mathrm{i}\mathbf{k}_\mathrm{a}\cdot\mathbf{r}}\hat{\mathbf{e}}_2 + x_3 \mathrm{e}^{\mathrm{i}\mathbf{k}_\mathrm{b}\cdot\mathbf{r}}\hat{\mathbf{e}}_3 + x_4 \mathrm{e}^{\mathrm{i}\mathbf{k}_\mathrm{b}\cdot\mathbf{r}}\hat{\mathbf{e}}_4 \qquad (6)$$

## Scattered Fields

Modelling them as point scatterers suspended in free space, the fields scattered by two particles P1 and P2 evaluated at some position vector $\mathbf{r}$ are,

$$\mathbf{E}_\mathrm{sca}^1(\mathbf{r}) = \frac{k_0^2}{\varepsilon_0}\overleftrightarrow{\mathbf{G}}(\mathbf{r}, \mathbf{r}_1)\mathbf{p}_1 \qquad (7a)$$

$$\mathbf{E}_\mathrm{sca}^2(\mathbf{r}) = \frac{k_0^2}{\varepsilon_0}\overleftrightarrow{\mathbf{G}}(\mathbf{r}, \mathbf{r}_2)\mathbf{p}_2 \qquad (7b)$$

Where $\mathbf{r}_1$ and $\mathbf{r}_2$ are the position vectors of P1 and P2, and $\mathbf{p}_1$ and $\mathbf{p}_2$ are the dipole moments at their centres. $\overleftrightarrow{\mathbf{G}}(\mathbf{r}, \mathbf{r}')$ is the dyadic Green's function evaluated at $\mathbf{r}$ with origin at $\mathbf{r}'$,

$$\overleftrightarrow{\mathbf{G}}(\mathbf{r}, \mathbf{r}') = \left[\overleftrightarrow{\mathbf{I}} - \frac{1}{k_0^2}\nabla\nabla\right]\frac{\mathrm{e}^{ik_0|\mathbf{r}-\mathbf{r}'|}}{4\pi|\mathbf{r}-\mathbf{r}'|} \qquad (8)$$

## Dipole Moments

A point dipole in one particle's centre is excited both by the incident field (6) and the field radiated by the other particle, (7a) or (7b). If P1 and P2 have diagonal polarizability tensors $\overleftrightarrow{\boldsymbol{\alpha}}_1$ and $\overleftrightarrow{\boldsymbol{\alpha}}_2$ respectively,

$$\mathbf{p}_1 = \overleftrightarrow{\boldsymbol{\alpha}}_1 \left( \mathbf{E}_{\text{inc}}(\mathbf{r}_1) + \frac{k_0^2}{\varepsilon_0} \overleftrightarrow{\mathbf{G}}(\mathbf{r}_1, \mathbf{r}_2)\mathbf{p}_2 \right) \quad (9a)$$

$$\mathbf{p}_2 = \overleftrightarrow{\boldsymbol{\alpha}}_2 \left( \mathbf{E}_{\text{inc}}(\mathbf{r}_2) + \frac{k_0^2}{\varepsilon_0} \overleftrightarrow{\mathbf{G}}(\mathbf{r}_2, \mathbf{r}_1)\mathbf{p}_1 \right) \quad (9b)$$

Beginning by substituting (9b) into (9a), these dipole moments can be re-written simply in terms of the incident field evaluated at $\mathbf{r}_1$ and $\mathbf{r}_2$, multiplied by an effective polarizability tensor,

$$\mathbf{p}_1 = \overleftrightarrow{\boldsymbol{\alpha}}_{\text{eff}}^{1,1} \mathbf{E}_{\text{inc}}(\mathbf{r}_1) + \overleftrightarrow{\boldsymbol{\alpha}}_{\text{eff}}^{1,2} \mathbf{E}_{\text{inc}}(\mathbf{r}_2) \quad (10a)$$

$$\mathbf{p}_2 = \overleftrightarrow{\boldsymbol{\alpha}}_{\text{eff}}^{2,1} \mathbf{E}_{\text{inc}}(\mathbf{r}_1) + \overleftrightarrow{\boldsymbol{\alpha}}_{\text{eff}}^{2,2} \mathbf{E}_{\text{inc}}(\mathbf{r}_2) \quad (10b)$$

Where $\overleftrightarrow{\boldsymbol{\alpha}}_{\text{eff}}^{m,n}$ refers to the effective polarizability in particle $m$ that acts on the electric field in particle $n$. These polarizabilities are given by,

$$\overleftrightarrow{\boldsymbol{\alpha}}_{\text{eff}}^{1,1} = \left[ \overleftrightarrow{\mathbf{I}} - \overleftrightarrow{\boldsymbol{\alpha}}_1 \frac{k_0^2}{\varepsilon_0} \overleftrightarrow{\mathbf{G}}(\mathbf{r}_1, \mathbf{r}_2) \overleftrightarrow{\boldsymbol{\alpha}}_2 \frac{k_0^2}{\varepsilon_0} \overleftrightarrow{\mathbf{G}}(\mathbf{r}_2, \mathbf{r}_1) \right]^{-1} \overleftrightarrow{\boldsymbol{\alpha}}_1 \quad (11a)$$

$$\overleftrightarrow{\boldsymbol{\alpha}}_{\text{eff}}^{1,2} = \left[ \overleftrightarrow{\mathbf{I}} - \overleftrightarrow{\boldsymbol{\alpha}}_1 \frac{k_0^2}{\varepsilon_0} \overleftrightarrow{\mathbf{G}}(\mathbf{r}_1, \mathbf{r}_2) \overleftrightarrow{\boldsymbol{\alpha}}_2 \frac{k_0^2}{\varepsilon_0} \overleftrightarrow{\mathbf{G}}(\mathbf{r}_2, \mathbf{r}_1) \right]^{-1} \overleftrightarrow{\boldsymbol{\alpha}}_1 \frac{k_0^2}{\varepsilon_0} \overleftrightarrow{\mathbf{G}}(\mathbf{r}_1, \mathbf{r}_2) \overleftrightarrow{\boldsymbol{\alpha}}_2 \quad (11b)$$

$$\overleftrightarrow{\boldsymbol{\alpha}}_{\text{eff}}^{2,1} = \left[ \overleftrightarrow{\mathbf{I}} - \overleftrightarrow{\boldsymbol{\alpha}}_2 \frac{k_0^2}{\varepsilon_0} \overleftrightarrow{\mathbf{G}}(\mathbf{r}_2, \mathbf{r}_1) \overleftrightarrow{\boldsymbol{\alpha}}_1 \frac{k_0^2}{\varepsilon_0} \overleftrightarrow{\mathbf{G}}(\mathbf{r}_1, \mathbf{r}_2) \right]^{-1} \overleftrightarrow{\boldsymbol{\alpha}}_2 \frac{k_0^2}{\varepsilon_0} \overleftrightarrow{\mathbf{G}}(\mathbf{r}_2, \mathbf{r}_1) \overleftrightarrow{\boldsymbol{\alpha}}_1 \quad (11c)$$

$$\overleftrightarrow{\boldsymbol{\alpha}}_{\text{eff}}^{2,2} = \left[ \overleftrightarrow{\mathbf{I}} - \overleftrightarrow{\boldsymbol{\alpha}}_2 \frac{k_0^2}{\varepsilon_0} \overleftrightarrow{\mathbf{G}}(\mathbf{r}_2, \mathbf{r}_1) \overleftrightarrow{\boldsymbol{\alpha}}_1 \frac{k_0^2}{\varepsilon_0} \overleftrightarrow{\mathbf{G}}(\mathbf{r}_1, \mathbf{r}_2) \right]^{-1} \overleftrightarrow{\boldsymbol{\alpha}}_2 \quad (11d)$$

## Total Electric Field

The total electric field at our cold spot's location, $\mathbf{r}_0$, is the sum of the fields scattered by the particles and the incident field,

$$\mathbf{E}_{\text{t}}(\mathbf{r}_0) = \frac{k_0^2}{\varepsilon_0} \overleftrightarrow{\mathbf{G}}(\mathbf{r}_0, \mathbf{r}_1)\mathbf{p}_1 + \frac{k_0^2}{\varepsilon_0} \overleftrightarrow{\mathbf{G}}(\mathbf{r}_0, \mathbf{r}_2)\mathbf{p}_2 + \mathbf{E}_{\text{inc}}(\mathbf{r}_0) \quad (12)$$

Equating (12) to (1), the total electric field developed when $x_i$ is the only non-zero amplitude in the incident field (6) is,

$$x_i\mathbf{E}_i(\mathbf{r}_0) = \frac{k_0^2}{\varepsilon_0}\overleftrightarrow{\mathbf{G}}(\mathbf{r}_0,\mathbf{r}_1)\mathbf{p}_1^{(x_i)} + \frac{k_0^2}{\varepsilon_0}\overleftrightarrow{\mathbf{G}}(\mathbf{r}_0,\mathbf{r}_2)\mathbf{p}_2^{(x_i)} + x_i\mathrm{e}^{\mathrm{i}\mathbf{k}_{\mathrm{a,b}}\cdot\mathbf{r}_0}\hat{\mathbf{e}}_i \qquad (13)$$

Where $\mathbf{p}_1^{(x_i)}$ and $\mathbf{p}_2^{(x_i)}$ are found by substituting $\mathbf{E}_{\mathrm{inc}}(\mathbf{r}) = x_i\mathrm{e}^{\mathrm{i}\mathbf{k}_{\mathrm{a,b}}\cdot\mathbf{r}}\hat{\mathbf{e}}_i$ into (10a) and (10b) and evaluating at the particle centres $\mathbf{r}_1$ and $\mathbf{r}_2$. Using (13) for each of the four incident field components, we can obtain the columns of the matrix $\overleftrightarrow{\mathbf{A}}$,

$$\mathbf{E}_1(\mathbf{r}_0) = \Bigg[\frac{k_0^2}{\varepsilon_0}\overleftrightarrow{\mathbf{G}}(\mathbf{r}_0,\mathbf{r}_1)\left(\overleftrightarrow{\boldsymbol{\alpha}}_{\mathrm{eff}}^{1,1}\mathrm{e}^{\mathrm{i}\mathbf{k}_{\mathrm{a}}\cdot\mathbf{r}_1} + \overleftrightarrow{\boldsymbol{\alpha}}_{\mathrm{eff}}^{1,2}\mathrm{e}^{\mathrm{i}\mathbf{k}_{\mathrm{a}}\cdot\mathbf{r}_2}\right) + \frac{k_0^2}{\varepsilon_0}\overleftrightarrow{\mathbf{G}}(\mathbf{r}_0,\mathbf{r}_2)\left(\overleftrightarrow{\boldsymbol{\alpha}}_{\mathrm{eff}}^{2,1}\mathrm{e}^{\mathrm{i}\mathbf{k}_{\mathrm{a}}\cdot\mathbf{r}_1} + \overleftrightarrow{\boldsymbol{\alpha}}_{\mathrm{eff}}^{2,2}\mathrm{e}^{\mathrm{i}\mathbf{k}_{\mathrm{a}}\cdot\mathbf{r}_2}\right) + \mathrm{e}^{\mathrm{i}\mathbf{k}_{\mathrm{a}}\cdot\mathbf{r}_0}\Bigg]\hat{\mathbf{e}}_1 \qquad (14a)$$

$$\mathbf{E}_2(\mathbf{r}_0) = \Bigg[\frac{k_0^2}{\varepsilon_0}\overleftrightarrow{\mathbf{G}}(\mathbf{r}_0,\mathbf{r}_1)\left(\overleftrightarrow{\boldsymbol{\alpha}}_{\mathrm{eff}}^{1,1}\mathrm{e}^{\mathrm{i}\mathbf{k}_{\mathrm{a}}\cdot\mathbf{r}_1} + \overleftrightarrow{\boldsymbol{\alpha}}_{\mathrm{eff}}^{1,2}\mathrm{e}^{\mathrm{i}\mathbf{k}_{\mathrm{a}}\cdot\mathbf{r}_2}\right) + \frac{k_0^2}{\varepsilon_0}\overleftrightarrow{\mathbf{G}}(\mathbf{r}_0,\mathbf{r}_2)\left(\overleftrightarrow{\boldsymbol{\alpha}}_{\mathrm{eff}}^{2,1}\mathrm{e}^{\mathrm{i}\mathbf{k}_{\mathrm{a}}\cdot\mathbf{r}_1} + \overleftrightarrow{\boldsymbol{\alpha}}_{\mathrm{eff}}^{2,2}\mathrm{e}^{\mathrm{i}\mathbf{k}_{\mathrm{a}}\cdot\mathbf{r}_2}\right) + \mathrm{e}^{\mathrm{i}\mathbf{k}_{\mathrm{a}}\cdot\mathbf{r}_0}\Bigg]\hat{\mathbf{e}}_2 \qquad (14b)$$

$$\mathbf{E}_3(\mathbf{r}_0) = \Bigg[\frac{k_0^2}{\varepsilon_0}\overleftrightarrow{\mathbf{G}}(\mathbf{r}_0,\mathbf{r}_1)\left(\overleftrightarrow{\boldsymbol{\alpha}}_{\mathrm{eff}}^{1,1}\mathrm{e}^{\mathrm{i}\mathbf{k}_{\mathrm{b}}\cdot\mathbf{r}_1} + \overleftrightarrow{\boldsymbol{\alpha}}_{\mathrm{eff}}^{1,2}\mathrm{e}^{\mathrm{i}\mathbf{k}_{\mathrm{b}}\cdot\mathbf{r}_2}\right) + \frac{k_0^2}{\varepsilon_0}\overleftrightarrow{\mathbf{G}}(\mathbf{r}_0,\mathbf{r}_2)\left(\overleftrightarrow{\boldsymbol{\alpha}}_{\mathrm{eff}}^{2,1}\mathrm{e}^{\mathrm{i}\mathbf{k}_{\mathrm{b}}\cdot\mathbf{r}_1} + \overleftrightarrow{\boldsymbol{\alpha}}_{\mathrm{eff}}^{2,2}\mathrm{e}^{\mathrm{i}\mathbf{k}_{\mathrm{b}}\cdot\mathbf{r}_2}\right) + \mathrm{e}^{\mathrm{i}\mathbf{k}_{\mathrm{b}}\cdot\mathbf{r}_0}\Bigg]\hat{\mathbf{e}}_3 \qquad (14c)$$

$$\mathbf{E}_4(\mathbf{r}_0) = \Bigg[\frac{k_0^2}{\varepsilon_0}\overleftrightarrow{\mathbf{G}}(\mathbf{r}_0,\mathbf{r}_1)\left(\overleftrightarrow{\boldsymbol{\alpha}}_{\mathrm{eff}}^{1,1}\mathrm{e}^{\mathrm{i}\mathbf{k}_{\mathrm{b}}\cdot\mathbf{r}_1} + \overleftrightarrow{\boldsymbol{\alpha}}_{\mathrm{eff}}^{1,2}\mathrm{e}^{\mathrm{i}\mathbf{k}_{\mathrm{b}}\cdot\mathbf{r}_2}\right) + \frac{k_0^2}{\varepsilon_0}\overleftrightarrow{\mathbf{G}}(\mathbf{r}_0,\mathbf{r}_2)\left(\overleftrightarrow{\boldsymbol{\alpha}}_{\mathrm{eff}}^{2,1}\mathrm{e}^{\mathrm{i}\mathbf{k}_{\mathrm{b}}\cdot\mathbf{r}_1} + \overleftrightarrow{\boldsymbol{\alpha}}_{\mathrm{eff}}^{2,2}\mathrm{e}^{\mathrm{i}\mathbf{k}_{\mathrm{b}}\cdot\mathbf{r}_2}\right) + \mathrm{e}^{\mathrm{i}\mathbf{k}_{\mathrm{b}}\cdot\mathbf{r}_0}\Bigg]\hat{\mathbf{e}}_4 \qquad (14d)$$
